# Supplementary material for: A longitudinal study of the top 1% toxic Twitter profiles
Source: arXiv:2303.14603 source file (2023-03-26)
Supplement: Supplementary file 1 [file appendix.tex]

\clearpage
\onecolumn
\section{Appendix}

\subsection{Perspective API Validation}

As a sanity check of the scores obtained from this API, we focused on the largest seed dataset, i.e., the ICWSM 2018~\cite{founta2018large}, and cross-correlated the scores from the API models with the annotations assigned to the tweet of a user based on the tweet content.
This dataset includes single tweets from 98.3K users, of which 4,940, 13,690, 27,094, and 52,652 were labeled as `hateful', `spam', `abusive', and `normal', respectively. We were able to retrieve tweets from the timelines of a total 39,344 users present in this dataset.
To validate that fact that pre-trained models of Perspective API's are producing stable outputs, we used the API models for ``Toxicity'',``Severe Toxicity'',``Identity Attack'',``Insult'',``Inflammatory'' and ``Threat'', because the definitions of these API scores are closest to the annotation effort from~\cite{founta2018large}.

For all users in the seed dataset, we computed the {\it median} 6 scores mentioned above across all of their tweets. The results of this investigation in Fig.~\ref{fig:api_validate} show the distribution of the API scores, for all four available annotations. Toxicity scores for abusive tweets have a median of 0.2 and highest score are 2.6. Hateful scores have highest value of 2.5. Normal and spam labeled tweets got very low Toxicity scores of 1.8 and 1.5 respectively. In all cases, the distributions of perspective score medians for users labeled ``abusive'' or ``hateful'' are significantly different (p\textless0.01) to those for users labeled ``normal'' or ``spam'', showing consistency between perspective scores and annotated user labels.

\begin{figure}[H]
 \centering
 \vspace{-0.5mm}
 \includegraphics[width=0.50\columnwidth]{figures/boxplot_labels.pdf}
 \caption{Distribution of scores from six Perspective API models vs. the human annotated labels of tweets.}
 \label{fig:api_validate}
\end{figure}
\subsection{Focus Profile Selection}

Focus group identification plots of Identity Attack Inflammatory, Insult and Threat scores are presented here. These groups were isolated by the imposing thresholds on respective median scores and Gini index. The details of the process can be found in (\S\ref{sec:focus-users}).
\label{all focus groups}
\begin{figure*}[h!]
\centering
{
\subfloat[Identity Attack]{
\includegraphics[width=0.24\textwidth]{sctr/IDENTITY_ATTACK_gini_median_hina.png}\label{fig}
}
\subfloat[Inflammatory]{
\includegraphics[width=0.24\textwidth]{sctr/INFLAMMATORY_gini_median_hina.png}\label{fig}
}
\subfloat[Insult]{
\includegraphics[width=0.24\textwidth]{sctr/INSULT_gini_median_hina.png}\label{fig:}
}
\subfloat[Threat]{
\includegraphics[width=0.24\textwidth]{sctr/THREAT_gini_median_hina.png}\label{fig:}
}
}
\caption{Focus profiles (bounded by the orange boxes), based on median and Gini coefficient of respective perspective scores of all 3T profiles.}
\label{fig:LABEL}
\end{figure*}
\subsection{URL analysis}

We plotted  the  top  20  categories  of  domains  out  of  all  different  categories  found in focus Identity Attack, focus Inflammatory, focus Insult and focus Threat profiles and their respective random sets of profiles in extension to the analysis performed in  ~\S\ref{sec:url-diversity}.  
\label{url analysis}
\begin{figure*}[t]
\centering
{
\subfloat[Identity Attack]{
\includegraphics[width=0.24\linewidth]{figures/bar_category_IDENTITY_ATTACK_median_xlog-crop.pdf}\label{fig:median:INFLAMMATORY-category}
}
\subfloat[Inflammatory]{
\includegraphics[width=0.24\linewidth]{figures/bar_category_INFLAMMATORY_median_xlog-crop.pdf}\label{fig:median:INFLAMMATORY-category}
}
\subfloat[Insult]{
\includegraphics[width=0.24\linewidth]{figures/bar_category_INSULT_median_xlog-crop.pdf}\label{fig:median:INSULT-2-category}
}
\subfloat[Threat]{
\includegraphics[width=0.24\linewidth]{figures/bar_category_THREAT_median_xlog-crop.pdf}\label{fig:median:THREAT-category}
}
}
\caption{Top 20 domain categories in focus and random Identity Attack, Inflammatory, Insult and Threat sets of profiles. Here, 2L-TLDs refer to second level domains (SLDs). 
``None'' refers to unrated websites whose domain category is unknown to FortiGuard.}
\vspace{-0.9mm}
\label{fig:bar_url_puser:gini_median-category_complete}
\end{figure*}
\newpage
\subsection{Coordination and Time Analysis}
Subplots in Figures~\ref{fig:day_week_gini_median_IDENTITY_ATTACK}~\ref{fig:day_week_gini_median_INFLAMMATORY},~\ref{fig:day_week_gini_median_INSULT} and~\ref{fig:day_week_gini_median_THREAT} are shared for focus Identity Attack, Inflammatory, Insult and Threat profiles and the respective random groups in extension to analysis performed in ~\ref{sec:tweeting-patterns}. Sub-plots (a) in these figures show the Probability Distribution Function (PDF) of time between sequential tweets by profiles of focus and random profiles, up to 60 minutes. Sub-plots(b) show the CDF of inter-tweet intervals as an extension to aforementioned PDF.
We also looked into the time of day and day of week at which tweets are posted by focus or random profiles across three types of misbehavior in sub-plots (c) and (d) of all four sets of figures.
\label{A:coordination analysis}

\begin{figure*}[h!]
    \vspace{-0.5mm}
    \begin{subfigure}[t]{0.24\linewidth}
            \includegraphics[width=\textwidth]{tsci/IDENTITY_ATTACK_gini_median_tbtH-small.pdf}
            \caption{Inter-tweet intervals}  \label{fig:}
    \end{subfigure}\hfill
      \begin{subfigure}[t]{0.24\linewidth}
            \includegraphics[width=\textwidth]{tsci/IDENTITY_ATTACK_gini_median_tbtC-small.pdf}
            \caption{Inter-tweet intervals}
    \label{fig:}
    \end{subfigure}
    \hfill
    \begin{subfigure}[t]{0.24\linewidth}
        \includegraphics[width=\textwidth]{tsci/IDENTITY_ATTACK_gini_median_DHnoOF-small.pdf}
            \caption{Tweets per hour}
            \label{fig:}
    \end{subfigure}
    \hfill
    \begin{subfigure}[t]{0.24\linewidth}
            \includegraphics[width=\textwidth]{tsci/IDENTITY_ATTACK_gini_median_DWDnoOF-small.pdf}
            \caption{Tweets per day}
            \label{fig:}
    \end{subfigure}
    % \caption{
    % Overview of temporal analysis: (a) PDF of tweet inter-arrival time;
    % (b) CDF of tweet inter-arrival time;
    % (c) PDF of tweet posting time during the day;
    % (d) PDF of tweet posting time during the week.
    % }
    \caption{Identity Attack}
    \label{fig:day_week_gini_median_IDENTITY_ATTACK}
    \vspace{-2mm}
\end{figure*}
\begin{figure*}[h!]
    \centering
    \begin{subfigure}{0.24\linewidth}
            \includegraphics[width=\textwidth]{tsci/INFLAMMATORY_gini_median_tbtH-small.pdf}
            \caption{Inter-tweet intervals} 
            \label{fig:}
    \end{subfigure}\hfill
     \begin{subfigure}{0.24\linewidth}
            \includegraphics[width=\textwidth]{tsci/INFLAMMATORY_gini_median_tbtC-small.pdf}
            \caption{Inter-tweet intervals} 
    \label{fig:}
    \end{subfigure}
    \begin{subfigure}{0.24\linewidth}
        \includegraphics[width=\textwidth]{tsci/INFLAMMATORY_gini_median_DHnoOF-small.pdf}
            \caption{Tweets per hour}
            \label{fig:}
    \end{subfigure}\hfill
    \begin{subfigure}{0.24\linewidth}
            \includegraphics[width=\textwidth]{tsci/INFLAMMATORY_gini_median_DWDnoOF-small.pdf}
            \caption{Tweets per day}
            \label{fig:}
    \end{subfigure}
    \caption{Inflammatory}
%     \caption{
%     INFLAMMATORY: Overview of temporal analysis: (a) PDF of tweet inter-arrival time;
%     (b) CDF of tweet inter-arrival time;
%     (c) PDF of tweet posting time during the day;
%     (d) PDF of tweet posting time during the week.
%  }
    \label{fig:day_week_gini_median_INFLAMMATORY}
\end{figure*}
\begin{figure*}[h!]
    \centering
    \begin{subfigure}{0.24\linewidth}
            \includegraphics[width=\textwidth]{tsci/INSULT_gini_median_tbtH-small.pdf}
            \caption{Inter-tweet intervals} 
            \label{fig:}
    \end{subfigure}\hfill
      \begin{subfigure}{0.24\linewidth}
            \includegraphics[width=\textwidth]{tsci/INSULT_gini_median_tbtC-small.pdf}
            \caption{Inter-tweet intervals} 
    \label{fig:}
    \end{subfigure}
    \begin{subfigure}{0.24\linewidth}
        \includegraphics[width=\textwidth]{tsci/INSULT_gini_median_DHnoOF-small.pdf}
            \caption{Tweets per hour}
            \label{fig:}
    \end{subfigure}\hfill
    \begin{subfigure}{0.24\linewidth}
            \includegraphics[width=\textwidth]{tsci/INSULT_gini_median_DWDnoOF-small.pdf}
            \caption{Tweets per day}
            \label{fig:}
    \end{subfigure}
    \caption{Insult}
%     \caption{
%     INSULT: Overview of temporal analysis: (a) PDF of tweet inter-arrival time;
%     (b) CDF of tweet inter-arrival time;
%     (c) PDF of tweet posting time during the day;
%     (d) PDF of tweet posting time during the week.
%  }
    \label{fig:day_week_gini_median_INSULT}
\end{figure*}
\begin{figure*}[h!]
    \centering
    \begin{subfigure}{0.24\linewidth}
            \includegraphics[width=\textwidth]{tsci/THREAT_gini_median_tbtH-small.pdf}
            \caption{Inter-tweet intervals} 
            \label{fig:}
    \end{subfigure}\hfill
     \begin{subfigure}{0.24\linewidth}
            \includegraphics[width=\textwidth]{tsci/THREAT_gini_median_tbtC-small.pdf}
            \caption{Inter-tweet intervals} 
    \label{fig:}
    \end{subfigure}
    \begin{subfigure}{0.24\linewidth}
        \includegraphics[width=\textwidth]{tsci/THREAT_gini_median_DHnoOF-small.pdf}
            \caption{Tweets per hour}
            \label{fig:}
    \end{subfigure}\hfill
    \begin{subfigure}{0.24\linewidth}
            \includegraphics[width=\textwidth]{tsci/THREAT_gini_median_DWDnoOF-small.pdf}
            \caption{Tweets per day}
            \label{fig:}
    \end{subfigure}
    \caption{Threat}
    \textbf{
    Overview of temporal analysis and coordination analysis: (a) PDF of tweet inter-arrival time;
    (b) CDF of tweet inter-arrival time;
    (c) PDF of tweet posting time during the day;
    (d) PDF of tweet posting time during the week.
}
    \label{fig:day_week_gini_median_THREAT}
    \end{figure*}
\subsection{Number of URLs and domains per focus and random profile}
\label{sec:no.url/domains}

In Figure~\ref{fig:urls and domains in tweets} we share the CDFs of the number of unique URLs and referenced domains in tweets of focus and random sets of profiles of all four types of investigated misbehavior such as Identity Attack, inflammatory and such (Section:~\ref{sec:url-diversity}).

\begin{figure*}[h!]
\centering
{
\subfloat[Identity Attack]{
\includegraphics[width=0.24\textwidth]{figures/domains_url_CDF_IDENTITY_ATTACK_median.pdf}\label{fig:}
}
\subfloat[Inflammatory]{
\includegraphics[width=0.24\textwidth]{figures/domains_url_CDF_INFLAMMATORY_median.pdf}\label{fig:}
}
\subfloat[Insult]{
\includegraphics[width=0.24\textwidth]{figures/domains_url_CDF_INSULT_median.pdf}\label{fig:}
}
\subfloat[Threat]{
\includegraphics[width=0.24\textwidth]{figures/domains_url_CDF_THREAT_median.pdf}\label{fig:}
}
}
\caption{CDFs of the Number of Unique URLs and Domains in Tweets of Focus and Random Group Profiles}
\label{fig:urls and domains in tweets}
\end{figure*}
\subsection{Number of hashtags per focus and random profile}
\label{sec:no.of hashtags}

Figure~\ref{fig:number of hashtags in tweets} represents the CDFs of the number of hashtags shared in tweets of focus and random profiles across all categories of misbehavior including Identity Attack, Inflammatory, Insult and Threat (Section:~\ref{sec:hashtag-diversity}).

\begin{figure*}[h!]
\centering
{
\subfloat[Identity Attack]{
\includegraphics[width=0.24\textwidth]{figures/hashtags_CDF_IDENTITY_ATTACK_median.pdf}\label{fig:}
}
\subfloat[Inflammatory]{
\includegraphics[width=0.24\textwidth]{figures/hashtags_CDF_INFLAMMATORY_median.pdf}\label{fig:}
}
\subfloat[Insult]{
\includegraphics[width=0.24\textwidth]{figures/hashtags_CDF_INSULT_median.pdf}\label{fig:}
}
\subfloat[Threat]{
\includegraphics[width=0.24\textwidth]{figures/hashtags_CDF_THREAT_median.pdf}\label{fig:}
}
}
\caption{CDFs of the Number of Unique Hashtags in Tweets of Focus and Random Group Profiles}
\label{fig:number of hashtags in tweets}
\end{figure*}
\subsection{URL Jaccard Similarity}

Figure~\ref{fig:domain similarity} furthers the results of Section ~\ref{sec:similarity-domains}  and Figure ~\S\ref{fig:url_domain_puser:gini_median-dom-simm} for the Perspective scores of Inflammatory, Insult, Threat and their respective random groups. The plots highlight the similarity of domains in focus and random groups and inter-similarity of domains found in tweets of focus and random groups across all four types of misbehavior.

\begin{figure*}[!]
\centering
{
\subfloat[Identity Attack]{
\includegraphics[width=0.24\textwidth]{figures/domains_similarity_IDENTITY_ATTACK_median_xlog.pdf}\label{fig:}
}
\subfloat[Inflammatory]{
\includegraphics[width=0.24\textwidth]{figures/domains_similarity_INFLAMMATORY_median_xlog.pdf}\label{fig:}
}
\subfloat[Insult]{
\includegraphics[width=0.24\textwidth]{figures/domains_similarity_INSULT_median_xlog.pdf}\label{fig:}
}
\subfloat[Threat]{
\includegraphics[width=0.24\textwidth]{figures/domains_similarity_THREAT_median_xlog.pdf}\label{fig:}
}
}
\caption{Domain Similarity among profiles of Focus and Random Profiles}
\label{fig:domain similarity}
\end{figure*}
\newpage
\subsection{Hashtag Jaccard Similarity}
These plots in Figure~\ref{fig:hashtags jaccard similarity} are shared to extend the results of Section ~\ref{sec:similarity-domains} for focus and random profiles of Inflammatory, Insult and Threat categories of misbehavior.

\begin{figure}[H]
\centering
{
\subfloat[Identity Attack]{
\includegraphics[width=0.24\textwidth]{figures/hashtags_jaccard_similarity_IDENTITY_ATTACK_median.pdf}\label{fig:}
}
\subfloat[Inflammatory]{
\includegraphics[width=0.24\textwidth]{figures/hashtags_jaccard_similarity_INFLAMMATORY_median.pdf}\label{fig:}
}
\subfloat[Insult]{
\includegraphics[width=0.24\textwidth]{figures/hashtags_jaccard_similarity_INSULT_median.pdf}\label{fig:}
}
\subfloat[Threat]{
\includegraphics[width=0.24\textwidth]{figures/hashtags_jaccard_similarity_THREAT_median.pdf}\label{fig:}
}
}
\caption{Jaccard
Similarity among Hashtags of Focus and Random Profiles}
\label{fig:hashtags jaccard similarity}
\end{figure}
\subsection{Hashtag Explanation}

% \setlength{\textfloatsep}{0pt}
% Table~\ref{tab:explain_hashtag} provides additional details about the unfamiliar hashtags that were previously highlighted in Tab.~\ref{tab:top5_htags_gini_median}. 
\begin{table*}[hb]
\resizebox{\textwidth}{!}{
\begin{tabular}{|l|l|}
\hline
Hashtag & Explanation \\
\hline
\#TreCru   & One Piece Treasure Cruise, a F2P RPG game   based on the popular manga and anime One Piece                 \\ \hline
\#BDS      & The Palestinian-led BDS movement promotes boycotts, divestments, and economic   sanctions against Israel \\ \hline
\#BREAKING & A hashtag used to represent breaking news.                                                                 \\ \hline
\#BlackLivesMatter & A political and social movement that seeks to highlight racism, discrimination, and inequality experienced by black people. \\ \hline
\#MeToo    & Me Too is a movement against sexual abuse and harassment through public disclosure of   allegations.     \\ \hline
\#MAGA     & Make America Great Again was a campaign slogan leading up to and during   the Trump presidency             \\ \hline
\#trap     & A subgenre of hip-hop music                                                                                \\ \hline
pg3d     & Pixel Gun 3D is a online multiplayer FPS heavily influenced by the pixel art style of Minecraft         \\ \hline
\end{tabular}
}
\caption{Explanations for lesser known hashtags that occur in Table~\ref{tab:top5_htags_gini_median}.}
\label{tab:explain_hashtag}
\end{table*}
